# Supplementary material for: Current fluctuations in nanopores reveal the polymer-wall adsorption potential
Source: arXiv:2012.00884 source file (2021-02-24)
Supplement: Supplementary file 1 [file SM.pdf]

# Supplemental material: Current fluctuations in nanopores reveal the polymer-wall adsorption potential

Stuart F Knowles, Nicole E Weckman, Vincent J Lim, Ulrich F Keyser, and Alice L Thorneywork
*Cavendish Laboratory, Department of Physics, University of Cambridge, JJ Thomson Avenue, Cambridge, CB3 0HE, United Kingdom*

Douwe J Bonthuis
*Institute of Theoretical and Computational Physics, Graz University of Technology, 8010 Graz, Austria*

(Dated: February 15, 2021)

## S1: EXPERIMENTAL DETAILS

Glass pores with a nominal diameter of 16nm are pulled from quartz glass capillaries with an inner/outer diameter of 0.2/0.5mm. Each chip contains 16 pulled capillaries arranged in a PDMS mould as two rows of 8 capillaries. All capillary tips (conical end) extend into a central reservoir with the opposite end of each capillary in its own separate reservoir on the edge of the chip. Following arrangement of the capillaries in the PDMS mould, chips are sealed onto a clean glass slide with more PDMS. To prepare for measurement assembled chips are plasma cleaned for five minutes, then the required measurement solution is injected through pre-punched holes in the PDMS. Complete filling of the pipettes is ensured by subsequently placing the chip under vacuum for a short period. Ag/AgCl Electrodes are inserted through the same holes used to inject solution, with the ground put into the central reservoir and the live electrode into the smaller side reservoir corresponding to a specific capillary. Current/Voltage curves are measured to verify the pore is functional, indicated by the resistance being in the correct range (c. 100M$\Omega$) for a 16nm pore in 500mM KCl, value varies with salt concentration) and by the response being smooth. This protocol allows for measurements to be performed separately on multiple different pores within the same chip to produce larger datasets.

All current-trace measurements are acquired with an Axopatch 200B patchclamp amplifier with data acquisition performed using a custom-built LabVIEW visual interface. Data was recorded at 250kHz with an analogue filter operating at 100kHz. This bandwidth was chosen to ensure that spectral data was acquired for all relevant frequencies without corruption by filter effects or aliasing. Power spectra were calculated from 3 minutes of current trace data then averaged over logarithmically spaced bins to improve precision. The minimum frequency component considered is c. 0.1Hz and the maximum is 5kHz. This frequency range is expected to capture all behaviour relevant to the transport properties of the pore; at lower frequencies noise is dominated by slow surface charge fluctuations, while above 5kHz noise is dominated by capacitative effects across the capillary wall.

For experiments with PEG in solution, the PEG concentration was such that the monomer density was constant between all experiments: 400$\mu$M PEG 1000, 50$\mu$M PEG 8000, 20$\mu$M PEG 20000. This corresponds to approximately 0.04%w/w PEG.

## S2: FULL SHAPE OF SPECTRA OVER ALL ACCESSIBLE FREQUENCIES

In figure S1, we present spectra for the system at 500mM KCl with and without PEG 8000 over the full range of frequencies accessible from our experiments. Different behaviour in different frequency regimes can be clearly identified; at low frequency ($f \lesssim$ 1Hz) the $1/f$ noise remains unchanged between spectra with and without PEG, at intermediate frequencies (1Hz $\lesssim f \lesssim$ 30kHz) we see an increase in spectral density with PEG, and at high frequencies ($>$ 30kHz), the spectra re-join each other before the spectral density is suppressed by the filter. In this high frequency regime the PSD was unchanged by adding PEG in all cases we measured. Although the precise values at which the spectra split and rejoin vary slightly from experiment to experiment, these values are typical of all systems studied

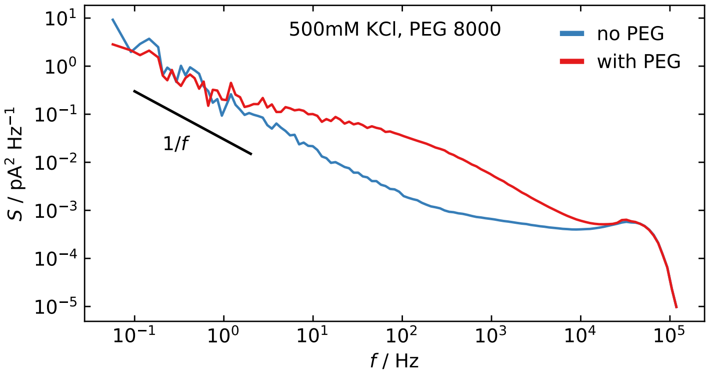


FIG. S1. A pair of spectra shown at full bandwidth. Data taken with PEG 8000 in 500mM KCl. It can be seen that the change in spectral density due to addition of PEG occurs over a finite bandwidth.

where we observe a change in noise upon addition of PEG.

## S3: DEPENDENCE OF $\Delta S$ ON PEG CONCENTRATION

To assess whether the experimental concentrations of PEG were in the regime of excess PEG, we repeated the nanopore measurement at 500mM KCl and PEG 1000 with 100× the concentration of PEG. In figure S2, we show the spectra at these two different concentrations. There is a degree of pore to pore variation, as evidenced by the difference between the blue curves in the two panels. Importantly however, the change in the spectrum on addition of PEG was comparable and certainly within this expected pore-to-pore variation, despite a 100 fold increase in PEG concentration. From this we conclude that PEG availability was not the limiting factor in our experiments.

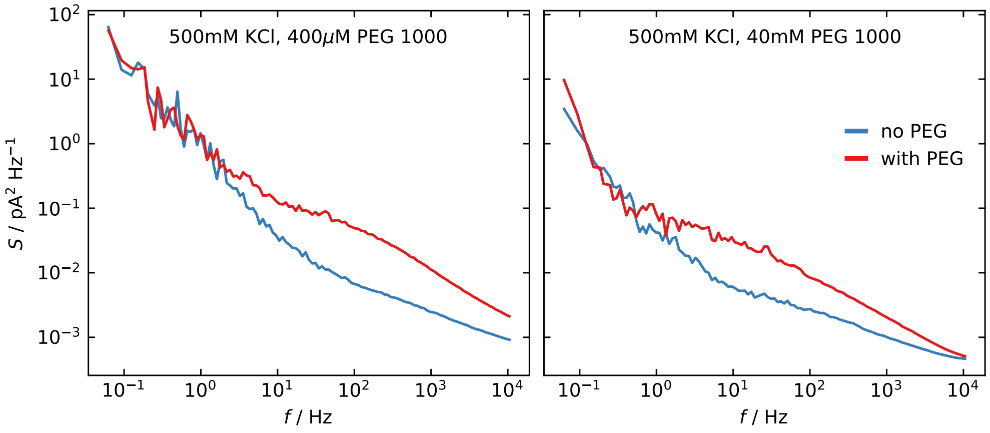


FIG. S2. A comparison of the change in the PSD for different concentrations of PEG. Despite expected variation in the intrinsic noise of each pore (blue curves), the change upon adding PEG (red curves) is comparable between the two cases, implying the PEG availability is not a limiting factor in our experiments.

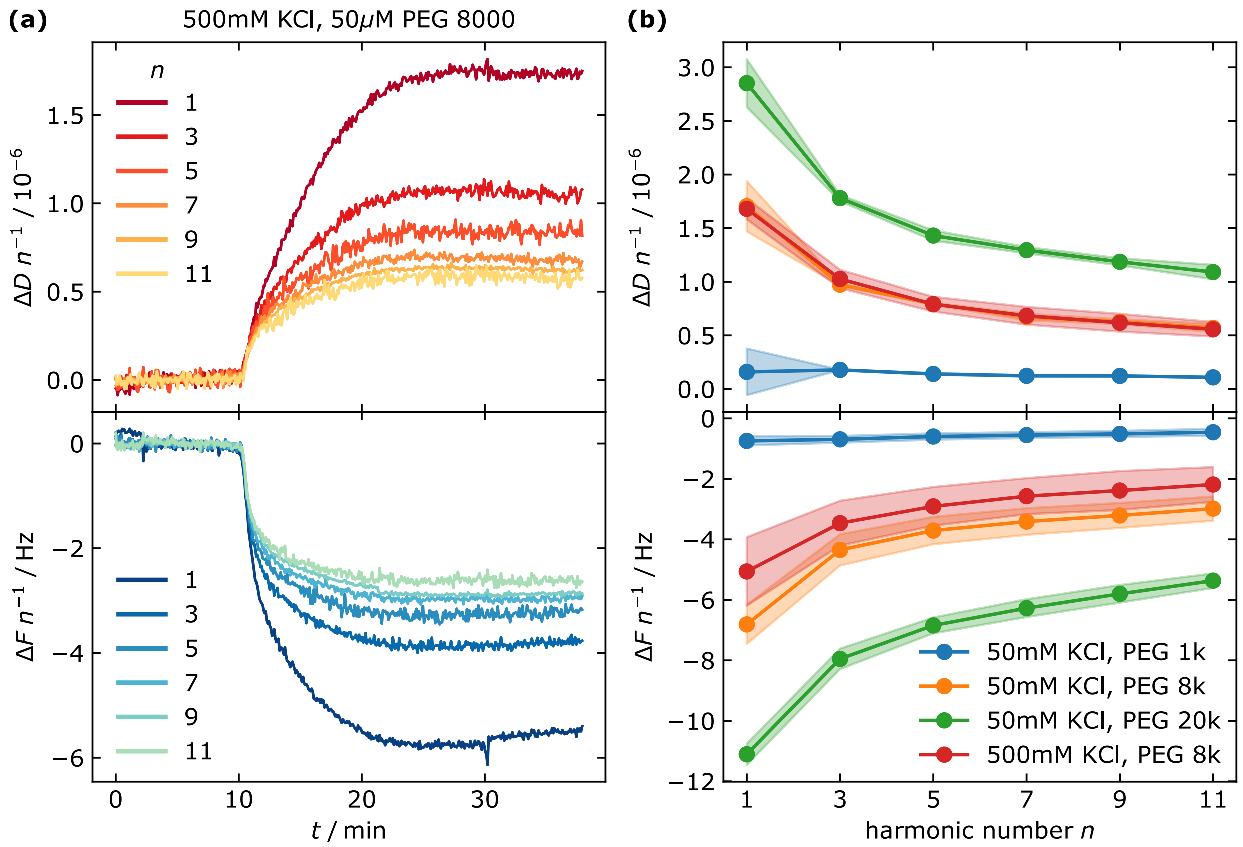


FIG. S3. (a) A full set of traces from a QCM-D experiment. The top panel shows the dissipation change, and the bottom panel shows the resonant frequency shift. (b) The equilibrium values for frequency shift and dissipation shift upon introduction of PEG, as a function of harmonic number. The uncertainties are shown as shaded areas.

## S4: QCM-D

The adsorption of PEG molecules onto glass surfaces is quantified using quartz crystal microbalance with dissipation monitoring (QCM-D). QCM-D experiments were performed in an E4 QCM-D unit from Q-Sense (Q-Sense AB, Göteborg, Sweden) using AT-cut quartz crystals (QSX303, $SiO_2$ surface) with a fundamental frequency of 5MHz. The crystals are first cleaned following standard protocols and then frequency and dissipation baselines are established by flowing the desired salt solution into the system. Solutions containing PEG at the same concentration as for the nanopore measurement are then flowed into the system and observed shifts in resonant frequency and dissipation are monitored for multiple harmonics of the fundamental frequency.

Figure S3 (a) shows a full set of traces for all harmonics as output by the Q-Sense software for adsorption of PEG 8000 in 500mM KCl. As is ubiquitous in QCM analysis, the curves are normalised by the harmonic number $n$. Note that in Fig. 2 of the main paper only the 3rd, 5th and 7th harmonics are shown as these are the most reliable; higher overtones have lower sensitivity and the fundamental is oversensitive to potentially spurious effects.

For a perfectly rigid adsorbed layer, the change in resonance frequency with adsorbed

mass is predicted to follow the Sauerbrey equation:

$$\frac{\Delta F_n}{n} = -\frac{m_f}{c}$$

with $\Delta F_n$ the frequency shift for a given harmonic, $n$ the harmonic number, $m_f$ the adsorbed mass per unit area, and $c$ a constant which depends only on the fundamental frequency of the crystal and the material properties of quartz. For our crystals, $c = 18\text{ng.cm}^{-2}.\text{Hz}^{-1}$.

The Sauerbrey equation predicts that for a perfectly rigid layer, the curves for different harmonics to collapse to a single curve. The fact that this is not true for our experimental data is the first indication of the viscoelastic character of the polymer layer.

For a more detailed comparison of data for experiments at different salt concentrations and with different PEG lengths, from each curve we extract values of $\Delta D$ and $\Delta F$ for long times where the curve has reached a plateau. Figure S3 (b) shows the values for frequency shift and dissipation shift for all harmonics and conditions. Importantly, in all cases values of $\Delta F$ are not zero, implying that we always have mass (polymer) adsorbing to the surface.

While the data for PEG 8000 at different salt concentrations is very similar, figure S3 (b) clearly shows that the value of $\Delta F$ increases with increasing PEG weight. Simple application of the Sauerbrey equation would suggest that this implies a greater mass of polymer is adsorbed for the larger PEG molecules. While we cannot exclude this possibility, the Sauerbrey equation is based on the assumption of a rigid and homogeneous adsorbed layer. The polymer layers in our experiments, however, clearly have viscoelastic character. Moreover, they are likely to have a relatively diffuse structure that may vary with polymer length, with fluid entrained in this layer also contributing to the measured frequency shift. As such, interpretation of the change in $\Delta F$ with PEG weight for our system is non-trivial. Moreover, we note that even if the mass of adsorbed polymer varies with PEG length, comparable power spectra are seen for systems with a 100-fold difference in the concentration of PEG (section S3).

While raw values of $\Delta D$ and $\Delta F$ are difficult to interpret, the ratio $\Delta D/\Delta F$ is a commonly used measure of the viscoelastic characteristics of the layer. This ratio is shown in figure S4 and is found to be very similar for all systems considered. As such, we conclude that the viscoelastic character of the layer does not vary significantly with PEG length or salt concentration.

## S5: FITTING PARAMETER $A$

When we scale our simulations to match the measured PSDs, we obtain a value of the amplitude scaling factor, $A$. As noted in the main text, this parameter is dependent on a number of different factors and variables, and is prohibitively difficult to predict from first principles. In Fig. S5 we present all of the values obtained for $A$:

This figure makes it clear that extracting any meaningful conclusions from the values of A would require more data, and is beyond the scope of this work. However, we do note the approximate $c^2$ scaling, which is consistent with a current blockage model, since in the range of salt concentrations we consider, current density near the wall scales with approximately

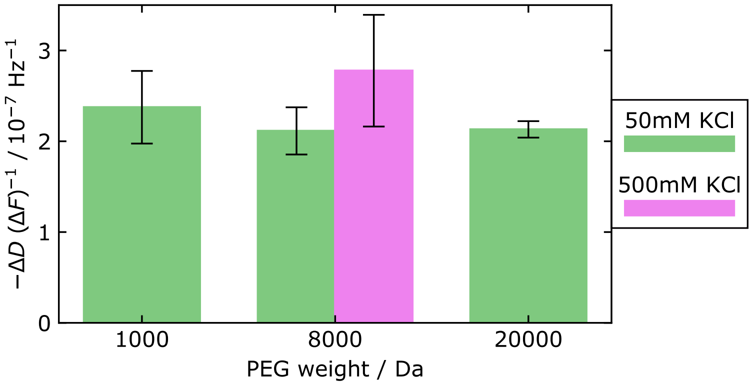


FIG. S4. The ratio $\Delta D/\Delta F$ for all parameter combinations considered. It is consistent across all parameters, implying that the character of the adsorbed layer is similar in all cases.

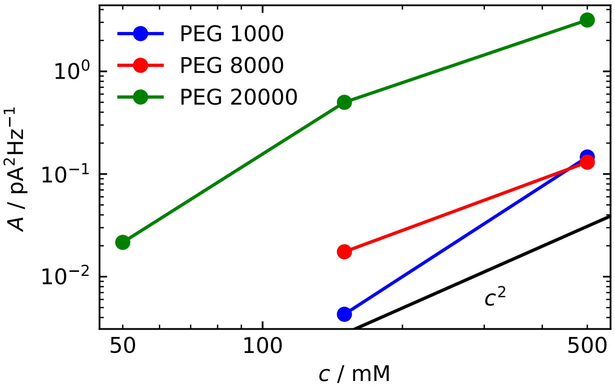


FIG. S5. The extracted values of A for all systems in which a change in spectral density was observed. A line of slope 2, corresponding to $c^2$ scaling, is shown as a guide, since at sufficiently high salt the surface current density scales with $c^2$.

$c$. If we were to investigate much lower salt concentrations we might expect this to level off as the current density becomes dominated by salt-independent Debye layer current density.

## S6: SIMULATION DETAILS

Here we present a more in-depth discussion of the implementation behind the simulations in our study. We simulate a cylindrical channel of length $L = 200\,\text{nm}$ and radius $R = 8\,\text{nm}$, connecting two reservoirs of $50 \times 50 \times 50\,\text{nm}^3$ each, as shown in Fig. S6 (a). Polymers suspended in a solvent undergo overdamped Brownian motion. For large times compared to the momentum relaxation time, the behaviour is diffusive. Diffusion of the polymers in the channel and the reservoirs is simulated by taking a number of test particles and generating one trial move for every particle at every simulation step $i$. The trial moves have a length $a = \sqrt{6\,D\,dt}\,\xi$ in each of the three directions, where $-1 < \xi < 1$ is a uniformly distributed random variable and $dt$ is the time interval of the step. This simulation scheme simulates diffusion with diffusion constant $D$ [1]. The position of a polymer at simulation step $i$ is

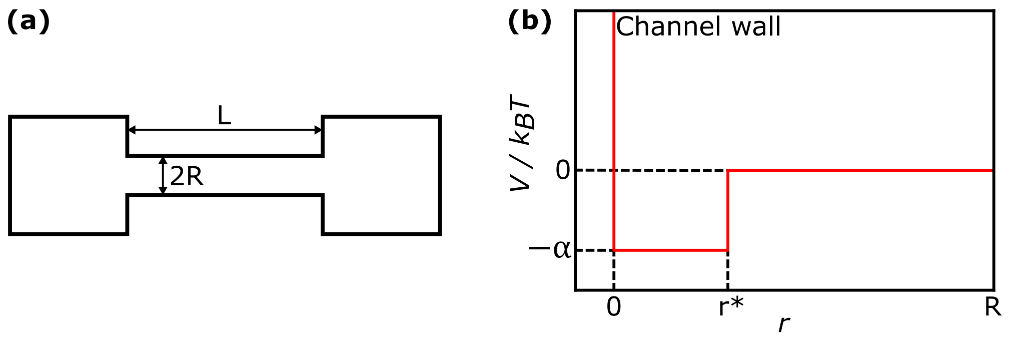


FIG. S6. Simulation schematics. (a) 2D cross-section of the system boundaries. (b) Adsorption potential within the channels.

denoted by $X_i = (x_i, y_i, z_i)$. Inside the channel, we define the coordinate $r$ in the radial direction, where $r = 0$ denotes the centre of the channel, and $r = R$ denotes the position of the channel wall. The adsorption potential is given by

$$V(X) = \begin{cases} \infty & \text{for } r < 0 \text{ and } -L/2 < z < L/2 \\ -\alpha & \text{for } 0 < r < r^* \text{ and } -L/2 < z < L/2 \\ 0 & \text{else,} \end{cases} \tag{1}$$

as shown in Fig. S6 (b).

The distance $r* \leq R$ denotes the range of the adsorption potential and $\alpha$ the depth, as shown in Fig. 4(a, inset) in the main text. Inside the adsorption zone ($r < r^*$, $-L/2 < z < L/2$), particles are immobilized. The particles desorb with a probability $\exp[-\alpha]$ if $X_{i+1}$ is outside the adsorption zone. This simulation protocol ensures that the ratio of adsorption and desorption rates is given by

$$\frac{k_{\text{on}}}{k_{\text{off}}} = e^{-\alpha}. \tag{2}$$

Furthermore, it naturally gives rise to a power-law distribution of residence times in the adsorption zone, in agreement with experimental results for PEG adsorption [2, 3].

For the global survey of different adsorption potentials, we have simulated at least $50\times10^6$ steps, and for the final curves in Fig. 4(b) of the main text, we have simulated $10^9$ steps, using 1000 test particles in the system. The diffusion coefficient has been set to $D = 35\,\text{nm}^2/\mu\text{s}$. Based on the Stokes-Einstein relation, this approximately corresponds to the diffusion coefficient of PEG20k molecules. For spherical objects of radius $R_g$ with no-slip boundary conditions, which is approprate for polymers [4], the friction coefficient equals $\gamma = 6\pi\eta R_g$. The momentum relaxation time equals $\tau = M/\gamma$, with $M$ being the molecular mass. For the PEG20k molecules, $\tau \approx 0.3$ fs, providing a lower boundary for the time step of the simulation. The maximum time step is given by setting the maximum step size equal to the particle radius, $\sqrt{6Ddt} = R_g$, giving $dt = 200$ ns. We have varied $dt$ in the simulations between 5 ns and 200 ns, and we have verified that the time step does not affect the results in this range.

The probability $p_{\text{ads}}(t)$ of the polymer being adsorbed at time $t = i\,dt$ is calculated as

the number of test particles in the adsorption zone as a fraction of the total number of test particles in the system. The power spectral density of $p_{\mathrm{ads}}(t)$ is denoted $S(f)$. We calculate the power spectrum using Welch's algorithm and FFT.

---


[1] K. Kikuchi, M. Yoshida, T. Maekawa, and H. Watanabe. Metropolis monte carlo method as a numerical technique to solve the fokker-planck equation. *Chem. Phys. Lett.*, 185:335, 1991.

[2] Michael J. Skaug, Joshua N. Mabry, and Daniel K. Schwartz. Single-molecule tracking of polymer surface diffusion. *J. Am. Chem. Soc.*, 136:1327–1332, 2014.

[3] Changqian Yu, Juan Guan, Kejia Chen, Sung Chul Bae, and Steve Granick. Single-molecule observation of long jumps in polymer adsorption. *ACS Nano*, 7:9735–9742, 2013.

[4] P.-G De Gennes. *Scaling concepts in polymer physics.* Cornell University Press, Ithaka, NY, 1979.
